# Supplementary material for: Dynamics of the non-classical light from a single solid-state quantum emitter
Source: arXiv:1209.3652 source file (2012-09-17)
Supplement: Supplementary file 1 [file DynamicG2-PRL-Supp-2_7.pdf]

# Supplement to
# Dynamics of the non-classical light from a single solid-state quantum emitter

Edward B. Flagg,* Sergey V. Polyakov, Tim Thomay, and Glenn S. Solomon†
*Joint Quantum Institute, National Institute of Standards and Technology,*
*& University of Maryland, Gaithersburg, MD, USA.*
(Dated: August 20, 2012)

In the manuscript we reported the dynamics of a second-order correlation function, $g^{(2)}_{\mathrm{HBT}}(t_1, t_2)$, where $t_1$ and $t_2$ are the delay times between the excitation pulse and photon detection on the two detectors. Here we develop the model used to produce the fits shown in Figs. 3(d)-(e) to the data in Figs. 3(a)-(b).

The second-order auto-correlation function recorded by a Hanbury Brown-Twiss measurement is defined as [1–3]

$$g^{(2)}_{\mathrm{HBT}}(t_1, t_2) = \frac{\left\langle \hat{a}^\dagger(t_1)\hat{a}^\dagger(t_2)\hat{a}(t_2)\hat{a}(t_1)\right\rangle}{\left\langle \hat{a}^\dagger(t_1)\hat{a}(t_1)\right\rangle \left\langle \hat{a}^\dagger(t_2)\hat{a}(t_2)\right\rangle}. \quad (1)$$

where $\hat{a}^\dagger$ and $\hat{a}$ are the photon creation and annihilation operators. The behavior of $g^{(2)}_{\mathrm{HBT}}(t_1, t_2)$ can be modeled by noting the equivalence between the expectation values of the photon operators and the elements of the density matrix of the semiconductor quantum dot (QD) (see [3] chap. 7):

$$\rho_{11}(t) = \left\langle \hat{a}^\dagger(t)\hat{a}(t)\right\rangle \quad (2a)$$
$$\rho_{00}(t) = \left\langle \hat{a}(t)\hat{a}^\dagger(t)\right\rangle \quad (2b)$$
$$\rho_{01}(t) = \left\langle \hat{a}^\dagger(t)\right\rangle \quad (2c)$$
$$\rho_{10}(t) = \left\langle \hat{a}(t)\right\rangle. \quad (2d)$$

where $\rho_{11}$ is the population of the QD state, $\rho_{00}$ is the population of the crystal ground state, and $\rho_{01} = \rho^*_{10}$ are the coherences between the states. The two factors in the denominator of Eqn. 1 are simply the QD population, $\rho_{11}(t)$, at different times, $t_1$ and $t_2$.

The behavior of the QD density matrix can be described with an exciton recapture model. Certain excitation wavelengths populate one or more reservoirs with carriers; for example, the GaAs conduction and valence bands for the 755 nm pump, or wetting layer states and an excited exciton state in the QD for the 893.0 nm pump. Over time these carriers either get captured in the QD or decay by other channels such as recombination through bulk exciton states or the wetting layer. For simplicity we only consider the lowest exciton energy level in the QD and assume that the decay of carriers in the reservoirs is unaffected by the presence of the QD. The density matrix equations of motion derived from the master equation for such an incoherently pumped system are

$$\frac{\mathrm{d}}{\mathrm{d}t}\rho_{11}(t) = f(t)\rho_{00}(t) - \Gamma_1\rho_{11}(t) \quad (3a)$$
$$\frac{\mathrm{d}}{\mathrm{d}t}\rho_{00}(t) = -f(t)\rho_{00}(t) + \Gamma_1\rho_{11}(t) \quad (3b)$$
$$\frac{\mathrm{d}}{\mathrm{d}t}\rho_{01}(t) = -\left(\frac{1}{2}\Gamma_1 + \Gamma_2\right)\rho_{01}(t) \quad (3c)$$
$$\frac{\mathrm{d}}{\mathrm{d}t}\rho_{10}(t) = -\left(\frac{1}{2}\Gamma_1 + \Gamma_2\right)\rho_{10}(t) \quad (3d)$$

where $f(t)$ is capture rate of carriers into the QD from the reservoirs, $\Gamma_1$ is the emission rate for the ground state exciton, and $\Gamma_2$ is the additional dephasing rate. See [4] for a similar set of evolution equations including the biexciton state.

The initial excitation pulse populates one or more reservoirs, and then the carrier population decays exponentially at different rates for each reservoir. The resulting expression for the capture rate is

$$f(t) = \sum_i \tilde{n}_i \exp\left(-\gamma_i t\right) \quad (4)$$

where $\tilde{n}_i$ is the product of the capture rate for a single carrier and the initial number of carriers in the $i^{th}$ reservoir, and $\gamma_i$ is the recombination rate of carriers in the $i^{th}$ reservoir. There may be several distinct decay paths with different values of $\tilde{n}_i$ and $\gamma_i$, such as the bulk exciton, defects in the vicinity of the QD, or the wetting layer.

To determine the values of the factors in the denominator of Eqn. 1 we need to solve for $\rho_{11}(t)$. We can use Eqns. 3 and the fact that the populations $\rho_{00}(t)$ and $\rho_{11}(t)$ sum to unity to obtain a single equation for the evolution of $\rho_{11}(t)$:

$$\frac{\mathrm{d}}{\mathrm{d}t}\rho_{11}(t) = f(t)\left[1 - \rho_{11}(t)\right] - \Gamma_1\rho_{11}(t). \quad (5)$$

We numerically integrate Eqn. 5 to determine $\rho_{11}(t)$ for all time after excitation.

Dealing with the numerator of Eqn. 1 is more complicated and requires the use of the quantum regression theorem [5, 6] which can be expressed as follows [7]. Given an expectation value of the form

$$\frac{\mathrm{d}}{\mathrm{d}t}\left\langle \hat{O}_j(t)\right\rangle = \sum_k L_{jk}(t)\left\langle \hat{O}_k(t)\right\rangle \quad (6)$$

then it is also true that

$$\frac{\mathrm{d}}{\mathrm{d}\tau}\left\langle \hat{A}(t)\hat{O}_j(t+\tau)\hat{B}(t)\right\rangle = \sum_k L_{jk}(t+\tau)\left\langle \hat{A}(t)\hat{O}_k(t+\tau)\hat{B}(t)\right\rangle, \tag{7}$$

where $\tau$ is the evolution time since $t$. By inspection of Eqns. 3, we can see that the density matrix elements are of the form of Eqn. 6. With the equivalences in Eqns. 2, we can use Eqn. 7 to derive the set of equations

$$\frac{\mathrm{d}}{\mathrm{d}\tau}G^{(2)}(t,\tau) = f(t+\tau)H^{(2)}(t,\tau) - \Gamma_1 G^{(2)}(t,\tau) \tag{8a}$$

$$\frac{\mathrm{d}}{\mathrm{d}\tau}H^{(2)}(t,\tau) = -f(t+\tau)H^{(2)}(t,\tau) + \Gamma_1 G^{(2)}(t,\tau) \tag{8b}$$

which are valid for $\tau \geq 0$ and where

$$G^{(2)}(t,\tau) = \left\langle \hat{a}^\dagger(t)\hat{a}^\dagger(t+\tau)\hat{a}(t+\tau)\hat{a}(t)\right\rangle \tag{9a}$$

$$H^{(2)}(t,\tau) = \left\langle \hat{a}^\dagger(t)\hat{a}(t+\tau)\hat{a}^\dagger(t+\tau)\hat{a}(t)\right\rangle. \tag{9b}$$

Note that $G^{(2)}(t,\tau)$ is the numerator of Eqn. 1 if we define $t_2 \equiv t_1+\tau$, and in the derivation of Eqns. 8 the coherences $\rho_{01}(t)$ and $\rho_{10}(t)$ were not needed. The irrelevance of the coherences can be understood by realizing that a Hanbury Brown-Twiss measurement is an intensity correlation of a single field, in contrast to correlation measurements performed on two intefering fields. To characterize the coherence of a non-classical state, a different measurement must be made. Thus in the manuscript we also perform a two-time Hong-Ou-Mandel cross-correlation measurement.

The initial conditions of Eqns. 8 at $\tau = 0$ are $G^{(2)}(t,0) = 0$ and $H^{(2)}(t,0) = \rho_{11}(t)$ which can be seen from their definitions and the properties of $\hat{a}$ and $\hat{a}^\dagger$. From Eqns. 8 we see that

$$\frac{\mathrm{d}}{\mathrm{d}\tau}G^{(2)}(t,\tau) = -\frac{\mathrm{d}}{\mathrm{d}\tau}H^{(2)}(t,\tau) \tag{10}$$

which when combined with the initial conditions implies conservation of the quantity

$$G^{(2)}(t,\tau) + H^{(2)}(t,\tau) = \rho_{11}(t) \tag{11}$$

for all $\tau$. Substituting this invariant expression into Eqns. 8 we obtain the expression

$$\frac{\mathrm{d}}{\mathrm{d}\tau}G^{(2)}(t,\tau) = f(t+\tau)\left(\rho_{11}(t) - G^{(2)}(t,\tau)\right) - \Gamma_1 G^{(2)}(t,\tau) \tag{12}$$

Numerically integrating Eqns. 5 and 12 and substituting the results into Eqn. 1, we can obtain a model correlation function

$$g^{(2)}_{\mathrm{HBT}}(t_1,t_2) = \frac{G^{(2)}(t_1,t_2-t_1)}{\rho_{11}(t_1)\rho_{11}(t_2)} \quad \text{for } t_2 \geq t_1. \tag{13}$$

To obtain the expression for $t_2 < t_1$, simply exchange $t_1$ and $t_2$ on the right-hand side of Eqn. 13.

An analysis of the limiting behavior of $g^{(2)}_{\mathrm{HBT}}(t_1,t_2)$ in Eqn. 13 shows that when $f(t) \approx \Gamma_1$, the source will be Poissonian except for a slice along $t_1 = t_2$ of width equal to the average capture time. In this slice $g^{(2)}_{\mathrm{HBT}}(t_1,t_2)$ ideally goes to zero, but will in practice be higher due to convolution with the detector response. In contrast, when $f(t) \ll \Gamma_1$ the source becomes perfectly antibunched, $g^{(2)}_{\mathrm{HBT}}(t_1,t_2) = 0$. The characteristic time scale for transition between the two limits is inversely proportional to the reservoir population decay, $1/\gamma_i$. Thus, if a quantum dot is excited via a carrier reservoir (either optically or electrically), a chance for multiple photon generation in a single excitation cycle will always be present. But the magnitude of the effect on overall multi-photon emission probability, defined as

$$P_{2+} = \frac{\iint G^{(2)}(t_1,t_2-t_1)\,\mathrm{d}t_1\,\mathrm{d}t_2}{\int\rho_{11}(t_1)\,\mathrm{d}t_1\int\rho_{11}(t_2)\,\mathrm{d}t_2}, \tag{14}$$

would be minimal for relatively fast reservoir decay, $\gamma_i \gg \Gamma_1$.

In the transition regime, the average time before additional capture increases as $f(t)$ decays. A cut of the $g^{(2)}_{\mathrm{HBT}}(t_1,t_2)$ surface along $t_2 = t_{\mathrm{const}} - t_1$ shows a dip, whose width grows exponentially with $t_{\mathrm{const}}$, as pumping due to the carrier reservoir $f(t)$ decays exponentially. At later times, when the system enters the $f(t) \ll \Gamma_1$ regime, the width of the dip becomes linear with $t_{\mathrm{const}}$, because subsequent captures become improbable.

We fit the model developed here to the $g^{(2)}_{\mathrm{HBT}}(t_1,t_2)$ data obtained in the experiment, with parameters from the measurements in Fig. 2 and including the effects of detector response time. See Table I for a list of model parameters.

* Electronic address: edward.flagg@nist.gov
† Electronic address: glenn.solomon@nist.gov

[1] R. Hanbury Brown and R. Q. Twiss, Nature **177**, 27 (1956).
[2] M. O. Scully and M. S. Zubairy, Quantum Optics (University Press, Cambridge, U. K., 1997).
[3] R. Loudon, The Quantum Theory of Light (Oxford U. Press, 2000), 3rd ed.
[4] E. Peter, S. Laurent, J. Bloch, J. Hours, S. Varoutsis, I. Robert-Philip, A. Beveratos, A. Lemaitre, A. Cavanna, G. Patriarche, et al., Applied Physics Letters **90**, 223118 (2007).
[5] L. Onsager, Phys. Rev. **37**, 405 (1931).
[6] M. Lax, Phys. Rev. **129**, 2342 (1963).
[7] J. I. Perea, D. Porras, and C. Tejedor, Phys. Rev. B **70**, 115304 (2004).

| Excitation wavelength | QD emission rate | Fast-decaying reservoir | | Slow-decaying reservoir | |
|---|---|---|---|---|---|
| $\lambda$ [nm] | $\Gamma_1$ [GHz] | $\gamma_1$ [GHz] | $\tilde{n}_1$ [GHz] | $\gamma_2$ [GHz] | $\tilde{n}_2$ [GHz] |
| 755 | 1.5 | 4.0 | 1.0 | 0.4 | 0.005 |
| 893.0 | 1.5 | 5.4 | 0.87 | - | - |

TABLE I: Simulation parameters for Fig. 3 (d) and (e) of the manuscript. $\Gamma_1$ is determined from streak camera measurements in Figs. 2 (b) and (c). Reservoir parameters are determined from a fit to the data presented in Figs. 3 (a) and (b).
